# Supplementary material for: sketch-plot: Progressive Editing for Text-to-Image Academic Figures
Source: arXiv:2606.09171 source file (2026-06-11)
Supplement: Supplementary file 1 [file appendix.tex]

\section{Ethical Considerations}
The dataset of 101 interactive documents was collected and utilized in strict compliance with applicable copyright regulations. To respect potential copyright concerns, we will only release the URLs of the collected documents rather than distributing their content. For our user study, we obtained explicit informed consent from all participants and rigorously anonymized all interview records to protect personal privacy. Although \system employs LLMs to assist in generation, we mitigate potential risks of AI hallucinations and uncontrollable outputs through a human-in-the-loop paradigm. By allowing users to review and edit the Document Specification (DocSpec) prior to code synthesis, customize styles via the Style Palette, and refine output through chat-based editing, the system ensures that creators retain full control over the authoring intent.

\begin{table}[htbp]
  \caption{Distribution of topics in \textsc{ViviBench} by subject area.}
  \label{tab:dataset}
  \begin{tabular}{lr}
    \toprule
    Subject Area & \# Topics \\
    \midrule
    Algorithms & 25 \\
    Mathematics & 24 \\
    Tools \& Resources & 13 \\
    Physics & 10 \\
    Science & 9 \\
    Other & 6 \\
    Explorable Explanations & 5 \\
    Systems \& Thought Experiments & 4 \\
    Psychology & 2 \\
    Creativity & 2 \\
    Books \& Essays & 1 \\
    \midrule
    \textbf{Total} & \textbf{101} \\
    \bottomrule
  \end{tabular}
\end{table}

\section{Interaction Taxonomy}
\label{app:taxonomy}

From the 101 collected documents, we extracted 482 interaction instances. Three visualization experts collaboratively classified these instances into 8 types based on interaction intent, inspired by Munzner's What-Why-How framework~\cite{munzner2014visualization}:

\begin{itemize}[nosep,leftmargin=*]
  \item \textbf{State Switching} (181, 37.6\%): Switching between discrete options, such as selecting a dataset, algorithm, or display mode.
  \item \textbf{Parameter Exploration} (121, 25.1\%): Adjusting continuous parameters to observe changes, such as tuning a slider for radius, frequency, or threshold.
  \item \textbf{Freeform Construction} (53, 11.0\%): Freely creating content, such as drawing shapes, writing code, editing values, or uploading files.
  \item \textbf{Direct Manipulation} (45, 9.3\%): Dragging objects within a visualization, such as data points, control points, or graph nodes.
  \item \textbf{Temporal Control} (32, 6.6\%): Controlling the time dimension, such as play/pause, stepping, speed adjustment, or timeline scrubbing.
  \item \textbf{Inspection} (24, 5.0\%): Exploring details on demand, such as hover tooltips or cursor tracking.
  \item \textbf{Spatial Navigation} (24, 5.0\%): Navigating in space, such as zooming, panning, or rotating 3D views.
  \item \textbf{Scroll-driven Narrative} (2, 0.4\%): Scrolling drives the narrative progression.
\end{itemize}

%%
%% SRTC Specs for the 8 Case Study Examples
%%
\section{SRTC Specifications for Case Study Examples}
\label{app:specs}

The following structured SRTC (State, Render, Transition, Constraint) specifications correspond to the eight interactive visualizations shown in Figure~\ref{fig:cases}. Each specification was produced by the \system Planner agent and served as the code-generation contract for the Executor.

\subsection*{(a) Parameter Exploration — The Lorenz Attractor}
\begin{table}[H]
  \small
  \centering
  \begin{tabularx}{\columnwidth}{@{}lX@{}}
\toprule
\textbf{S} & \texttt{sigma}: slider $[1, 30]$, default 10; \texttt{rho}: slider $[10, 60]$, default 28; \texttt{beta}: constant 2.667; \texttt{trajectory}: derived numerical integration of $dx/dt=\sigma(y-x), dy/dt=x(\rho-z)-y, dz/dt=xy-\beta z$ \\
\midrule
\textbf{R} & \textbullet~A continuously growing 3D phase-space trajectory projected onto a 2D canvas \newline \textbullet~The trail fades over time to emphasize recent motion \newline \textbullet~A slow auto-rotation of the view around the vertical axis \newline \textbullet~Two sliders for $\sigma$ and $\rho$ displayed below the canvas \\
\midrule
\textbf{T} & \textbullet~Adjusting the $\sigma$ slider resets the trajectory and restarts integration from the same initial point \newline \textbullet~Adjusting the $\rho$ slider resets the trajectory, causing the attractor shape to deform or collapse into a stable orbit \\
\midrule
\textbf{C} & For classical values ($\sigma=10$, $\rho=28$, $\beta=8/3$), the trajectory never repeats and draws a distinctive butterfly-shape---demonstrating sensitive dependence on initial conditions. \\
\bottomrule
  \end{tabularx}
\end{table}

\subsection*{(b) Direct Manipulation — Geometric Optics Ray Tracing}
\begin{table}[H]
  \small
  \centering
  \begin{tabularx}{\columnwidth}{@{}lX@{}}
\toprule
\textbf{S} & \texttt{object\_x}: drag-x $[20, \text{lens\_x} - 10]$; \texttt{object\_y}: drag-y $[0, \text{canvas\_height}]$; \texttt{f}: drag-x $[40, 300]$; \texttt{u}: derived $\text{lens\_x} - \text{object\_x}$; \texttt{v}: derived $(u \cdot f) / (u - f)$; \texttt{M}: derived $v / u$; \texttt{image\_type}: derived if $v>0$: Real Inverted, if $v<0$: Virtual Upright, if $v=\infty$: Undefined \\
\midrule
\textbf{R} & \textbullet~A central convex lens whose thickness scales with focal length \newline \textbullet~An orange draggable object arrow on the left of the lens \newline \textbullet~Two green draggable focal points $F$ and $F'$ on the optical axis \newline \textbullet~Three principal rays drawn from the object tip through the lens \newline \textbullet~A colored image arrow on the right (green for real, blue for virtual) \newline \textbullet~An instrument dashboard showing live values of $f, u, v$, and $M$ \newline \textbullet~A status tag indicating image type and orientation \\
\midrule
\textbf{T} & \textbullet~Dragging the orange object arrow horizontally changes $u$ and updates all derived optical values \newline \textbullet~Dragging the object arrow vertically changes the object height and redraws the ray diagram \newline \textbullet~Dragging a focal point ($F$ or $F'$) changes $f$, reshaping both the lens and all derived values simultaneously \\
\midrule
\textbf{C} & The thin lens equation $1/u + 1/v = 1/f$ is always satisfied. When $u < f$, the image distance $v$ becomes negative (virtual image). When $u = f$, the image forms at infinity. \\
\bottomrule
  \end{tabularx}
\end{table}

\subsection*{(c) Inspection — Voronoi Tessellation}
\begin{table}[H]
  \small
  \centering
  \begin{tabularx}{\columnwidth}{@{}lX@{}}
\toprule
\textbf{S} & \texttt{seeds}: 15 points initialized at random positions, moving with slow random velocity; \texttt{mouse\_pos}: hover; \texttt{nearest}: derived $\arg\min_k d(\text{mouse\_pos}, \text{seeds}[k])$; \texttt{min\_dist}: derived $d(\text{mouse\_pos}, \text{seeds}[\text{nearest}])$; \texttt{cell\_region}: derived all pixels closest to \texttt{seeds[nearest]} within 150px from \texttt{mouse\_pos} \\
\midrule
\textbf{R} & \textbullet~An animated canvas of 15 slowly drifting seed points on a dark background \newline \textbullet~On hover: the hovered Voronoi cell illuminated with a purple radial gradient \newline \textbullet~On hover: a dashed gold line connecting the cursor to its nearest seed \newline \textbullet~On hover: a transparent circle of radius \texttt{min\_dist} visualizing the nearest-neighbor envelope \newline \textbullet~The nearest seed highlighted in gold; all others remain purple \\
\midrule
\textbf{T} & \textbullet~Moving the mouse over the canvas updates \texttt{mouse\_pos} continuously \newline \textbullet~Each frame recalculates the nearest seed and updates the illuminated cell, connecting line, and envelope circle in real-time \\
\midrule
\textbf{C} & The illuminated region always corresponds exactly to the Voronoi cell of the nearest seed. Every point within the highlighted region is provably closer to that seed than to any other---demonstrating the core definition of Voronoi partitioning. \\
\bottomrule
  \end{tabularx}
\end{table}

\subsection*{(d) Freeform Construction — Neural Network Forward Propagation}
\begin{table}[H]
  \small
  \centering
  \begin{tabularx}{\columnwidth}{@{}lX@{}}
\toprule
\textbf{S} & \texttt{hidden\_nodes}: click-to-place list of $\{x, y\}$, default $[]$; \texttt{weights}: derived random initialization; \texttt{activations}: derived forward pass (sigmoid); \texttt{output\_val}: derived average of output neuron activations \\
\midrule
\textbf{R} & \textbullet~Three fixed red input nodes ($x_1, x_2, x_3$) on the left \newline \textbullet~Two fixed blue output nodes ($y_1, y_2$) on the right \newline \textbullet~User-placed yellow hidden nodes in the central region \newline \textbullet~Directed arrows connecting all layers; animate green (input$\to$hidden) then orange (hidden$\to$output) during forward pass \newline \textbullet~Activation values displayed on each node \newline \textbullet~An output activation progress bar and percentage readout \newline \textbullet~A 'Send Signal' button and a 'Clear' button \\
\midrule
\textbf{T} & \textbullet~Clicking in the central canvas zone places a new hidden neuron and immediately triggers an animated forward pass \newline \textbullet~Pressing 'Send Signal' replays the forward pass with newly randomized weights \newline \textbullet~Pressing 'Clear' removes all hidden nodes and resets the output bar to 50\% \\
\midrule
\textbf{C} & Adding more hidden neurons generally introduces more non-linearity. The output activation always falls in $(0, 1)$ due to the sigmoid function, regardless of network topology. \\
\bottomrule
  \end{tabularx}
\end{table}

\subsection*{(e) Scroll-driven Narrative — Thermodynamic Entropy}
\begin{table}[H]
  \small
  \centering
  \begin{tabularx}{\columnwidth}{@{}lX@{}}
\toprule
\textbf{S} & \texttt{scroll\_progress}: scroll-wheel $[0, 1]$, default 0; \texttt{partition\_y}: derived $\text{scroll\_progress} \times \text{canvas\_height}$; \texttt{particles}: 150 red + 150 blue bouncing particles; \texttt{entropy\_S}: derived fraction of particles that have crossed to the other side times 100 \\
\midrule
\textbf{R} & \textbullet~A dark split-canvas with 300 bouncing particles: red on left, blue on right \newline \textbullet~A central vertical wall separating the two halves, present only from \texttt{partition\_y} downward \newline \textbullet~A live entropy counter ($S = \dots$) displayed in red in the top-left corner \newline \textbullet~A scroll-progress fill bar on the left edge \\
\midrule
\textbf{T} & \textbullet~Scrolling downward increases \texttt{scroll\_progress}, raising \texttt{partition\_y} and shortening the wall from the top, allowing particles to mix \newline \textbullet~Scrolling upward decreases \texttt{scroll\_progress}, lowering \texttt{partition\_y} and re-blocking particle passage \\
\midrule
\textbf{C} & As the wall is removed ($\text{scroll\_progress} \to 1$), particles irreversibly mix---entropy $S$ increases monotonically. The constraint $\Delta S \ge 0$ maps directly to the unidirectional scroll interaction, visualizing time's arrow. \\
\bottomrule
  \end{tabularx}
\end{table}

\subsection*{(f) Spatial Navigation — The Möbius Strip}
\begin{table}[H]
  \small
  \centering
  \begin{tabularx}{\columnwidth}{@{}lX@{}}
\toprule
\textbf{S} & \texttt{rotX}: drag-y $[-3.14, 3.14]$, default 0.5; \texttt{rotY}: drag-x $[-3.14, 3.14]$, default -0.5; \texttt{surface}: derived parametric mesh $x(u,v)=(R+v\cos(u/2))\cos(u), y(u,v)=v\sin(u/2), z(u,v)=(R+v\cos(u/2))\sin(u)$ \\
\midrule
\textbf{R} & \textbullet~A 3D polygon mesh of the Möbius strip rendered using the Painter's Algorithm \newline \textbullet~Faces colored with a teal-to-sky-blue gradient mapped to the $u$ parameter \newline \textbullet~Depth shading simulating a diffuse light source \newline \textbullet~Numeric overlays showing the current \texttt{rotX} and \texttt{rotY} viewing angles \\
\midrule
\textbf{T} & \textbullet~Clicking and dragging horizontally on the canvas updates \texttt{rotY}, rotating the strip around the vertical axis \newline \textbullet~Clicking and dragging vertically updates \texttt{rotX}, tilting the strip forward or backward \newline \textbullet~Releasing the mouse locks the current orientation \\
\midrule
\textbf{C} & No matter how the strip is rotated, a continuous path along its surface always returns to the starting point in a mirrored orientation, demonstrating the strip's single-sidedness. \\
\bottomrule
  \end{tabularx}
\end{table}

\subsection*{(g) State Switching — Quantum Electron Orbitals}
\begin{table}[H]
  \small
  \centering
  \begin{tabularx}{\columnwidth}{@{}lX@{}}
\toprule
\textbf{S} & \texttt{orbital\_state}: segmented-button [\texttt{1s}, \texttt{2p}, \texttt{3d}], default \texttt{1s}; \texttt{wavefunction}: derived $\psi(r,\theta) = \text{radial\_part}(n,l) \times \text{angular\_part}(l,m)$; \texttt{density\_cloud}: derived Monte Carlo sampling, accept point $(x,y)$ with probability $\propto |\psi(x,y)|^2$ \\
\midrule
\textbf{R} & \textbullet~A 2D canvas with coordinate axes and a nucleus dot at the origin \newline \textbullet~Points progressively sampled and plotted, accumulating into a probability density cloud \newline \textbullet~A wavefunction equation display that updates to reflect the active orbital state \newline \textbullet~A segmented button control with options \texttt{1s}, \texttt{2p}, and \texttt{3d} \\
\midrule
\textbf{T} & \textbullet~Clicking a segment button sets \texttt{orbital\_state} to the selected orbital \newline \textbullet~Switching state clears all existing sample points and triggers a new Monte Carlo sampling run \\
\midrule
\textbf{C} & Each orbital state produces a distinct, characteristic spatial density pattern: \texttt{1s} is spherically symmetric, \texttt{2p} is a dumbbell shape with a nodal plane, and \texttt{3d} forms a four-lobed clover pattern---matching theoretical predictions. \\
\bottomrule
  \end{tabularx}
\end{table}

\subsection*{(h) Temporal Control — Fourier Series Epicycles}
\begin{table}[H]
  \small
  \centering
  \begin{tabularx}{\columnwidth}{@{}lX@{}}
\toprule
\textbf{S} & \texttt{time}: playback $[0, \infty]$, default 0; \texttt{is\_playing}: toggle, default true; \texttt{n\_harmonics}: slider $[1, 15]$ (step 2), default 5; \texttt{wave}: derived last 500 $y$-values of the epicycle tip \\
\midrule
\textbf{R} & \textbullet~A chain of rotating circles (epicycles), each at a frequency proportional to its harmonic index \newline \textbullet~A dot tracing the tip of the outermost epicycle \newline \textbullet~A reconstructed square wave drawn on the right by recording the tip's $y$-position over time \newline \textbullet~A dashed line connecting the epicycle tip to the leading edge of the wave \newline \textbullet~A Play/Pause button and a harmonic count slider \\
\midrule
\textbf{T} & \textbullet~Pressing Play/Pause starts or freezes the rotation of all epicycles \newline \textbullet~Dragging the harmonic slider adds or removes outer epicycles in odd increments, immediately reshaping the output wave \\
\midrule
\textbf{C} & As \texttt{n\_harmonics} increases toward infinity, the reconstructed wave converges to a perfect square wave, demonstrating Fourier's theorem that any periodic signal decomposes into sinusoids. \\
\bottomrule
  \end{tabularx}
\end{table}
